# Supplementary material for: FittedGenes: Domain-Aware Sewing Pattern Layout Optimization
Source: arXiv:2611.28022 source file (2026-09-27)
Supplement: Supplementary file 1 [file supplementary-VMV2026-sub.tex]

% ---------------------------------------------------------------------------
% Supplementary material driver — VMV 2026 submission
% Mirrors the structure of EGauthorGuidelines-VMV2026-sub.tex exactly.

\documentclass{egpubl}
\usepackage{VMV2026}

\WsSubmission

% !! *please* don't change anything above
% !! unless you REALLY know what you are doing
% ------------------------------------------------------------------------
\usepackage[T1]{fontenc}
\usepackage{dfadobe}

\usepackage{cite}
\BibtexOrBiblatex
\electronicVersion
\PrintedOrElectronic
\ifpdf \usepackage[pdftex]{graphicx} \pdfcompresslevel=9
\else \usepackage[dvips]{graphicx} \fi

\usepackage{egweblnk}
% end of prologue

% -----------------------------------------------------------------------
% Paper-specific packages
% -----------------------------------------------------------------------
\usepackage{color}
\newcommand{\MK}[1]{{\color{orange}[\textbf{MK:} #1]}}
\newcommand{\AB}[1]{{\color{blue}[\textbf{AB:} #1]}}
\usepackage{amsmath}
\usepackage{amssymb}
\usepackage{booktabs}
\usepackage{float}
\usepackage{multirow}
\usepackage{url}
\usepackage{algorithm}
\usepackage{algpseudocode}
\usepackage{placeins}
\usepackage{longtable}
\usepackage{tabularx}
\usepackage{array}

\newcolumntype{Y}{>{\centering\arraybackslash}X}

\usepackage{cleveref}
\crefname{figure}{Fig.}{Figs.}
\Crefname{figure}{Fig.}{Figs.}
\crefname{table}{Tab.}{Tabs.}
\Crefname{table}{Tab.}{Tabs.}
\crefname{section}{Sec.}{Secs.}
\Crefname{section}{Section}{Sections}
\crefname{equation}{Eq.}{Eqs.}
\Crefname{equation}{Eq.}{Eqs.}
\crefname{app}{App.}{Apps.}
\Crefname{app}{App.}{Apps.}
\setcounter{secnumdepth}{3} % number down to \subsubsection, but not \paragraph

\input{supplementary-body-sub.inc}
